# Supplementary material for: Ab Initio Finite Temperature Auxiliary Field Quantum Monte Carlo
Source: arXiv:1806.02848 ancillary file (2018-08-14)
Supplement: Supplementary file 1 [file supplementary-material-ab.pdf]

# Supplement: *Ab Initio* Finite Temperature Auxiliary Field Quantum Monte Carlo

Yuan Liu, Minsik Cho, and Brenda Rubenstein\*

Department of Chemistry, Brown University, Providence Rhode Island 02912, USA

## A. The Continuous Hubbard-Stratonovich Transformation of an *Ab Initio* Hamiltonian

In this section, we provide more details regarding the manipulation of the *ab initio* Hamiltonian that makes it amenable to a continuous Hubbard-Stratonovich Transformation. As described in the main text, after recasting the two body interaction term into a density-density form, a supermatrix,  $V_{(i\alpha,k\alpha),(l\beta,j\beta)}$  may be formed and diagonalized (or decomposed) into

$$V_{(i\alpha,k\alpha),(l\beta,j\beta)} = \sum_{\gamma}^{(2N)^2} R_{(i\alpha,k\alpha)\gamma} \lambda_{\gamma} R_{(l\beta,j\beta)\gamma}^*, \quad (1)$$

where  $\lambda_{\gamma}$  is the  $\gamma$ -th eigenvalue, and  $R_{(i\alpha,k\alpha)\gamma}$  is the  $(i\alpha,k\alpha)$ -th element of the  $\gamma$ -th eigenvector. The two body term then becomes

$$\begin{aligned} \frac{1}{2} \sum_{i\alpha,j\beta,k\alpha,l\beta}^{2N} V_{(i\alpha,k\alpha),(j\beta,l\beta)} c_{i\alpha}^{\dagger} c_{k\alpha} c_{j\beta}^{\dagger} c_{l\beta} &= \frac{1}{2} \sum_{i\alpha,j\beta,k\alpha,l\beta}^{2N} \sum_{\gamma}^{(2N)^2} R_{(i\alpha,k\alpha)\gamma} \lambda_{\gamma} R_{(l\beta,j\beta)\gamma}^* (c_{i\alpha}^{\dagger} c_{k\alpha}) (c_{j\beta}^{\dagger} c_{l\beta}) \\ &= \frac{1}{2} \sum_{\gamma}^{(2N)^2} \lambda_{\gamma} \left( \sum_{i\alpha,k\alpha}^{2N} R_{(i\alpha,k\alpha)\gamma} (c_{i\alpha}^{\dagger} c_{k\alpha}) \right) \left( \sum_{j\beta,l\beta}^{2N} R_{(l\beta,j\beta)\gamma}^* (c_{j\beta}^{\dagger} c_{l\beta}) \right), \end{aligned} \quad (2)$$

where the creation and annihilation operators follow the definition in the main text.

Following Zhang, it may be recognized that  $\sum_{j\beta,l\beta}^{2N} R_{(l\beta,j\beta)\gamma}^* (c_{j\beta}^{\dagger} c_{l\beta})$  and  $\sum_{i\alpha,k\alpha}^{2N} R_{(i\alpha,k\alpha)\gamma} (c_{i\alpha}^{\dagger} c_{k\alpha})$  are simply Hermitian conjugates of each other. We can therefore write the two body potential operator,  $\hat{V}$ , as

$$\hat{V} = \frac{1}{2} \sum_{\gamma}^{(2N)^2} \lambda_{\gamma} \hat{\rho}_{\gamma} \hat{\rho}_{\gamma}^{\dagger} - \frac{1}{2} \sum_{\alpha} \hat{\rho}_0^{\alpha}, \quad (3)$$

where

$$\hat{\rho}_{\gamma} = \sum_{i\alpha,k\alpha}^{2N} R_{(i\alpha,k\alpha)\gamma} (c_{i\alpha}^{\dagger} c_{k\alpha}), \quad (4)$$

and

$$\hat{\rho}_0^{\alpha} = \sum_{ij}^N \left( \sum_k^N V_{ikkj}^{\alpha\alpha\alpha\alpha} \right) c_{i\alpha}^{\dagger} c_{j\alpha}. \quad (5)$$

It is straightforward to see that Hermiticity guarantees that

$$\hat{\rho}_{\gamma} \hat{\rho}_{\gamma}^{\dagger} = \hat{\rho}_{\gamma}^{\dagger} \hat{\rho}_{\gamma}. \quad (6)$$

It follows that Equation (3) may be re-expressed as

---

\* brenda\_rubenstein@brown.edu

$$\hat{V} = \frac{1}{4} \sum_{\gamma}^{(2N)^2} \lambda_{\gamma} \{\hat{\rho}_{\gamma}, \hat{\rho}_{\gamma}^{\dagger}\} - \frac{1}{2} \sum_{\alpha} \hat{\rho}_0^{\alpha} \quad (7)$$

$$= \frac{1}{8} \sum_{\gamma}^{(2N)^2} \lambda_{\gamma} [(\hat{\rho}_{\gamma} + \hat{\rho}_{\gamma}^{\dagger})^2 - (\hat{\rho}_{\gamma} - \hat{\rho}_{\gamma}^{\dagger})^2] - \frac{1}{2} \sum_{\sigma} \hat{\rho}_0^{\sigma}. \quad (8)$$

$\hat{\rho}_0^{\alpha}$  is a one body term and can be readily combined with the original one body term  $\hat{K}$ . The total Hamiltonian may now be expressed as

$$\hat{H} = \sum_{\alpha} \hat{H}_{1\alpha} + \hat{H}_2, \quad (9)$$

in which

$$\hat{H}_{1\alpha} = \sum_{ij}^N T_{i\alpha,j\alpha} \hat{c}_{i\alpha}^{\dagger} \hat{c}_{j\alpha} - \mu \sum_i^N \hat{c}_{i\alpha}^{\dagger} \hat{c}_{i\alpha} - \frac{1}{2} \hat{\rho}_0^{\alpha}, \quad (10)$$

$$\hat{H}_2 = \frac{1}{8} \sum_{\gamma}^{(2N)^2} \lambda_{\gamma} [(\hat{\rho}_{\gamma} + \hat{\rho}_{\gamma}^{\dagger})^2 - (\hat{\rho}_{\gamma} - \hat{\rho}_{\gamma}^{\dagger})^2]. \quad (11)$$

Observe that  $\hat{H}_2$  is now a summation of squares of one body terms, and can be decoupled using the continuous Hubbard-Stratonovich Transformation in the following way

$$\begin{aligned} e^{-\Delta\tau \hat{H}_2} &= e^{-\frac{\Delta\tau}{8} \sum_{\gamma}^{(2N)^2} \lambda_{\gamma} (\hat{\rho}_{\gamma} + \hat{\rho}_{\gamma}^{\dagger})^2} e^{\frac{\Delta\tau}{8} \sum_{\gamma}^{(2N)^2} \lambda_{\gamma} (\hat{\rho}_{\gamma} - \hat{\rho}_{\gamma}^{\dagger})^2} \\ &= \prod_{\gamma}^{(2N)^2} \left( \frac{1}{\sqrt{2\pi}} \right)^2 \int_{-\infty}^{\infty} \int_{-\infty}^{\infty} d\phi_{\gamma-} d\phi_{\gamma+} e^{-\frac{\phi_{\gamma+}^2 + \phi_{\gamma-}^2}{2}} e^{i\frac{\sqrt{\Delta\tau\lambda_{\gamma}}}{2} \phi_{\gamma+} (\hat{\rho}_{\gamma} + \hat{\rho}_{\gamma}^{\dagger})} e^{\frac{\sqrt{\Delta\tau\lambda_{\gamma}}}{2} \phi_{\gamma-} (\hat{\rho}_{\gamma} - \hat{\rho}_{\gamma}^{\dagger})}. \end{aligned} \quad (12)$$

The propagator can be further split into the spin up and down contributions,

$$\hat{B}_{\uparrow}(\phi_{\gamma+}, \phi_{\gamma-}) \hat{B}_{\downarrow}(\phi_{\gamma+}, \phi_{\gamma-}) = e^{i\frac{\sqrt{\Delta\tau\lambda_{\gamma}}}{2} \phi_{\gamma+} (\hat{\rho}_{\gamma} + \hat{\rho}_{\gamma}^{\dagger})} e^{\frac{\sqrt{\Delta\tau\lambda_{\gamma}}}{2} \phi_{\gamma-} (\hat{\rho}_{\gamma} - \hat{\rho}_{\gamma}^{\dagger})}, \quad (13)$$

where

$$\hat{B}_{\uparrow}(\phi_{\gamma+}, \phi_{\gamma-}) = e^{i\frac{\sqrt{\Delta\tau\lambda_{\gamma}}}{2} \phi_{\gamma+}} \left( \sum_{i\uparrow,k\uparrow}^N R_{(i\uparrow,k\uparrow)\gamma} c_{i\uparrow}^{\dagger} c_{k\uparrow} + \sum_{i\uparrow,k\uparrow}^N R_{(i\uparrow,k\uparrow)\gamma}^* c_{k\uparrow}^{\dagger} c_{i\uparrow} \right) e^{\frac{\sqrt{\Delta\tau\lambda_{\gamma}}}{2} \phi_{\gamma-}} \left( \sum_{i\uparrow,k\uparrow}^N R_{(i\uparrow,k\uparrow)\gamma} c_{i\uparrow}^{\dagger} c_{k\uparrow} - \sum_{i\uparrow,k\uparrow}^N R_{(i\uparrow,k\uparrow)\gamma}^* c_{k\uparrow}^{\dagger} c_{i\uparrow} \right) \quad (14)$$

$$\hat{B}_{\downarrow}(\phi_{\gamma+}, \phi_{\gamma-}) = e^{i\frac{\sqrt{\Delta\tau\lambda_{\gamma}}}{2} \phi_{\gamma+}} \left( \sum_{i\downarrow,k\downarrow}^N R_{(i\downarrow,k\downarrow)\gamma} c_{i\downarrow}^{\dagger} c_{k\downarrow} + \sum_{i\downarrow,k\downarrow}^N R_{(i\downarrow,k\downarrow)\gamma}^* c_{k\downarrow}^{\dagger} c_{i\downarrow} \right) e^{\frac{\sqrt{\Delta\tau\lambda_{\gamma}}}{2} \phi_{\gamma-}} \left( \sum_{i\downarrow,k\downarrow}^N R_{(i\downarrow,k\downarrow)\gamma} c_{i\downarrow}^{\dagger} c_{k\downarrow} - \sum_{i\downarrow,k\downarrow}^N R_{(i\downarrow,k\downarrow)\gamma}^* c_{k\downarrow}^{\dagger} c_{i\downarrow} \right) \quad (15)$$

are the up and down propagators for one site within one imaginary time step, respectively. Putting this altogether, the total propagator for one imaginary time step for the spin sector  $\alpha$  is

$$\hat{B}_{\alpha}(\vec{\phi}) = e^{-\frac{\Delta\tau \hat{H}_{1\alpha}}{2}} \left[ \prod_{\gamma=1}^{(2N)^2} \hat{B}_{\alpha}(\phi_{\gamma+}, \phi_{\gamma-}) \right] e^{-\frac{\Delta\tau \hat{H}_{1\alpha}}{2}}, \alpha = \{\uparrow, \downarrow\}. \quad (16)$$

## B. Details of the Background Subtraction

To reduce the phase problem, we can further subtract  $\langle \hat{\rho}_{\gamma} + \hat{\rho}_{\gamma}^{\dagger} \rangle$  and  $\langle \hat{\rho}_{\gamma} - \hat{\rho}_{\gamma}^{\dagger} \rangle$  from (11). In this case, the two body term becomes

$$\frac{1}{8} \sum_{\gamma}^{(2N)^2} \lambda_{\gamma} [(\hat{\rho}_{\gamma} + \hat{\rho}_{\gamma}^{\dagger})^2 - (\hat{\rho}_{\gamma} - \hat{\rho}_{\gamma}^{\dagger})^2] = \hat{H}_2 + \frac{1}{4} \hat{\eta}_+ - \frac{1}{4} \hat{\eta}_- - \frac{1}{8} \hat{\eta}_0, \quad (17)$$

where

$$\hat{H}_2 = \frac{1}{8} \sum_{\gamma}^{(2N)^2} \lambda_{\gamma} \left\{ [(\hat{\rho}_{\gamma} + \hat{\rho}_{\gamma}^{\dagger}) - \langle \hat{\rho}_{\gamma} + \hat{\rho}_{\gamma}^{\dagger} \rangle]^2 - [(\hat{\rho}_{\gamma} - \hat{\rho}_{\gamma}^{\dagger}) - \langle \hat{\rho}_{\gamma} - \hat{\rho}_{\gamma}^{\dagger} \rangle]^2 \right\} \quad (18)$$

$$\hat{\eta}_+ = \sum_{\gamma}^{(2N)^2} \lambda_{\gamma} \langle \hat{\rho}_{\gamma} + \hat{\rho}_{\gamma}^{\dagger} \rangle (\hat{\rho}_{\gamma} + \hat{\rho}_{\gamma}^{\dagger}), \quad (19)$$

$$\hat{\eta}_- = \sum_{\gamma}^{(2N)^2} \lambda_{\gamma} \langle \hat{\rho}_{\gamma} - \hat{\rho}_{\gamma}^{\dagger} \rangle (\hat{\rho}_{\gamma} - \hat{\rho}_{\gamma}^{\dagger}), \quad (20)$$

$$\hat{\eta}_0 = \sum_{\gamma}^{(2N)^2} \lambda_{\gamma} \left( \langle \hat{\rho}_{\gamma} + \hat{\rho}_{\gamma}^{\dagger} \rangle^2 - \langle \hat{\rho}_{\gamma} - \hat{\rho}_{\gamma}^{\dagger} \rangle^2 \right). \quad (21)$$

$\hat{\eta}_+$  and  $\hat{\eta}_-$  are one body terms, which can be combined with  $\hat{H}_1$  in (10). The constant term  $\hat{\eta}_0$  can be ignored because it won't affect the physical observables in the sampling process.

After simplification, the total Hamiltonian is therefore

$$\hat{H} = \sum_{\alpha} \hat{H}_{1\alpha} + \hat{H}_2, \quad (22)$$

with

$$\hat{H}_{1\alpha} = \sum_{ij}^N T_{i\alpha, j\alpha} \hat{c}_{i\alpha}^{\dagger} \hat{c}_{j\alpha} - \frac{1}{2} \hat{\rho}_0^{\alpha} - \mu \sum_i \hat{c}_{i\alpha}^{\dagger} \hat{c}_{i\alpha} + \frac{1}{2} \sum_{\gamma}^{(2N)^2} \lambda_{\gamma} \langle \hat{\rho}_{\gamma} \rangle \hat{\rho}_{\gamma}^{\dagger\alpha} + \frac{1}{2} \sum_{\gamma}^{(2N)^2} \lambda_{\gamma} \langle \hat{\rho}_{\gamma}^{\dagger} \rangle \hat{\rho}_{\gamma}^{\alpha}, \quad (23)$$

and  $\hat{H}_2$  is given in (18). The additional superscript  $\alpha$  in  $\hat{\rho}_{\gamma}^{\alpha}$  and  $\hat{\rho}_{\gamma}^{\dagger\alpha}$  means we only pick out the corresponding one-body portion with the correct spin index from the total  $\hat{\rho}_{\gamma}$  and  $\hat{\rho}_{\gamma}^{\dagger}$  to combine into  $\hat{H}_{1\alpha}$ . As described above, we can then proceed to decouple  $\hat{H}_2$  using a continuous HS transform, and calculate the partition function and observables of interest.

### C. Details of Importance Sampling

Starting from (18), after applying the continuous Hubbard-Stratonovich Transformation as in (12), the two body propagator containing the background subtraction term now becomes

$$e^{-\Delta\tau\hat{H}_2} = \prod_{\gamma}^{(2N)^2} \left( \frac{1}{\sqrt{2\pi}} \right)^2 \int_{-\infty}^{\infty} \int_{-\infty}^{\infty} d\phi_{\gamma-} d\phi_{\gamma+} e^{-\frac{\phi_{\gamma+}^2 + \phi_{\gamma-}^2}{2}} e^{i\frac{\sqrt{\Delta\tau\lambda_{\gamma}}}{2} \phi_{\gamma+} [(\hat{\rho}_{\gamma} + \hat{\rho}_{\gamma}^{\dagger}) - \langle \hat{\rho}_{\gamma} + \hat{\rho}_{\gamma}^{\dagger} \rangle]} e^{\frac{\sqrt{\Delta\tau\lambda_{\gamma}}}{2} \phi_{\gamma-} [(\hat{\rho}_{\gamma} - \hat{\rho}_{\gamma}^{\dagger}) - \langle \hat{\rho}_{\gamma} - \hat{\rho}_{\gamma}^{\dagger} \rangle]}. \quad (24)$$

Introducing a force bias shift to every auxiliary field in the above equation, we obtain

$$\begin{aligned} e^{-\Delta\tau\hat{H}_2} &= \prod_{\gamma}^{(2N)^2} \left( \frac{1}{\sqrt{2\pi}} \right)^2 \int_{-\infty}^{\infty} \int_{-\infty}^{\infty} d\phi_{\gamma-} d\phi_{\gamma+} e^{-\frac{(\phi_{\gamma+} - \bar{\phi}_{\gamma+})^2 + (\phi_{\gamma-} - \bar{\phi}_{\gamma-})^2}{2}} e^{i\frac{\sqrt{\Delta\tau\lambda_{\gamma}}}{2} (\phi_{\gamma+} - \bar{\phi}_{\gamma+}) [(\hat{\rho}_{\gamma} + \hat{\rho}_{\gamma}^{\dagger}) - \langle \hat{\rho}_{\gamma} + \hat{\rho}_{\gamma}^{\dagger} \rangle]} \times \\ &\quad e^{\frac{\sqrt{\Delta\tau\lambda_{\gamma}}}{2} (\phi_{\gamma-} - \bar{\phi}_{\gamma-}) [(\hat{\rho}_{\gamma} - \hat{\rho}_{\gamma}^{\dagger}) - \langle \hat{\rho}_{\gamma} - \hat{\rho}_{\gamma}^{\dagger} \rangle]} \\ &= \prod_{\gamma}^{(2N)^2} \left( \frac{1}{\sqrt{2\pi}} \right)^2 \int_{-\infty}^{\infty} \int_{-\infty}^{\infty} d\phi_{\gamma-} d\phi_{\gamma+} p(\phi_{\gamma+}, \phi_{\gamma-}) W'(\phi_{\gamma+}, \bar{\phi}_{\gamma+}, \phi_{\gamma-}, \bar{\phi}_{\gamma-}) \hat{B}(\phi_{\gamma+} - \bar{\phi}_{\gamma+}, \phi_{\gamma-} - \bar{\phi}_{\gamma-}), \end{aligned} \quad (25)$$

where

$$W'(\phi_{\gamma+}, \bar{\phi}_{\gamma+}, \phi_{\gamma-}, \bar{\phi}_{\gamma-}) = e^{-\frac{\bar{\phi}_{\gamma+}^2 + \bar{\phi}_{\gamma-}^2}{2}} e^{\bar{\phi}_{\gamma+} \phi_{\gamma+} + \bar{\phi}_{\gamma-} \phi_{\gamma-}}, \quad (26)$$

contributes to the overall weight of each walker.

### D. Obtaining Mean Field Trial Density Matrices and Energies

Observables from mean field theory (MFT) are evaluated using a finite temperature mean field density matrix, which also serves as the trial density matrix for our quantum Monte Carlo simulations. Here, we provide more details on how mean field density matrices are obtained. We can approximate the two body portion of the *ab initio* Hamiltonian by introducing a mean field density matrix,  $\bar{D}_{ij}^\alpha$ , to obtain

$$\frac{1}{2} \sum_{\alpha\beta} \sum_{ijkl}^N V_{ijkl}^{\alpha\beta\alpha\beta} \hat{c}_{i\alpha}^\dagger \hat{c}_{k\alpha} \hat{c}_{j\beta}^\dagger \hat{c}_{l\beta} = \frac{1}{2} \sum_{\alpha\beta} \sum_{ijkl}^N V_{ijkl}^{\alpha\beta\alpha\beta} (\hat{c}_{i\alpha}^\dagger \hat{c}_{k\alpha} - \bar{D}_{ik}^\alpha) (\hat{c}_{j\beta}^\dagger \hat{c}_{l\beta} - \bar{D}_{jl}^\beta) + \frac{1}{2} \sum_{\alpha} (\hat{\rho}_{MF1}^\alpha + \hat{\rho}_{MF2}^\alpha) - \frac{1}{2} \hat{\rho}_{MF0}, \quad (27)$$

where  $\hat{\rho}_{MF1}^\alpha$ ,  $\hat{\rho}_{MF2}^\alpha$  and  $\hat{\rho}_{MF0}$  are the one body and constant terms,

$$\hat{\rho}_{MF1}^\alpha = \sum_{ik} \left( \sum_{jl}^N \sum_{\beta} V_{ijkl}^{\alpha\beta\alpha\beta} \bar{D}_{jl}^\beta \right) \hat{c}_{i\alpha}^\dagger \hat{c}_{k\alpha}, \quad (28)$$

$$\hat{\rho}_{MF2}^\alpha = \sum_{ik} \left( \sum_{jl}^N \sum_{\beta} V_{jilk}^{\beta\alpha\beta\alpha} \bar{D}_{jl}^\beta \right) \hat{c}_{i\alpha}^\dagger \hat{c}_{k\alpha}; \quad (29)$$

$$\hat{\rho}_{MF0} = \sum_{\alpha\beta} \sum_{ijkl}^N V_{ijkl}^{\alpha\beta\alpha\beta} \bar{D}_{ik}^\alpha \bar{D}_{jl}^\beta. \quad (30)$$

The one body terms may be combined with the kinetic operator, while the constant term can be added at the end of any total energy calculation.

Invoking the mean field approximation means that we ignore the remaining two body term  $\frac{1}{2} \sum_{\alpha\beta} \sum_{ijkl}^N V_{ijkl}^{\alpha\beta\alpha\beta} (\hat{c}_{i\alpha}^\dagger \hat{c}_{k\alpha} - \bar{D}_{ik}^\alpha) (\hat{c}_{j\beta}^\dagger \hat{c}_{l\beta} - \bar{D}_{jl}^\beta)$ , which is a small contribution representing the deviation of the system from the mean field solution. This yields the final mean field Hamiltonian

$$\hat{H}_{MF} = \sum_{\alpha} \sum_{ij}^N T_{i\alpha,j\alpha} \hat{c}_{i\alpha}^\dagger \hat{c}_{j\alpha} - \frac{1}{2} \sum_{\alpha} \hat{\rho}_0^\alpha + \frac{1}{2} \sum_{\alpha} (\hat{\rho}_{MF1}^\alpha + \hat{\rho}_{MF2}^\alpha) - \frac{1}{2} \hat{\rho}_{MF0}, \quad (31)$$

which can be solved easily at finite temperature to obtain its related mean field density matrix  $\bar{D}_{ij}^\alpha$ . This density matrix can then be used to construct a new Hamiltonian  $\hat{H}_{MF}$  given by (31). To obtain the final mean field density matrix, we therefore must iterate this procedure until we achieve convergence: first, we obtain an estimate of the density matrix, then, we form a new Hamiltonian, then, we obtain a new estimate of the density matrix, and so on. When this process is finished, we arrive at a self-consistent mean field solution for  $\bar{D}_{ij}^\alpha$ , which we can use as a trial density matrix for performing background subtraction, or from which we can directly measure observables. Note that at low temperature, the self-consistent process may be difficult to converge. We use a linear density mixing scheme to improve the convergence.

### E. Proof of the Positive Semi-Definiteness of the *Ab Initio* Supermatrix

Elements of an *ab initio* supermatrix  $\mathbf{V}$  are defined by

$$V_{(i\alpha,k\alpha),(l\beta,j\beta)} = \int d\vec{r}_1 d\vec{r}_2 \phi_{i\alpha}^*(\vec{r}_1) \phi_{j\beta}^*(\vec{r}_2) \frac{1}{|\vec{r}_1 - \vec{r}_2|} \phi_{k\alpha}(\vec{r}_1) \phi_{l\beta}(\vec{r}_2), \quad (32)$$

where  $\vec{r}_i$  represents the spatial coordinates of the  $i$ -th electron, and  $\phi_{i\alpha}$  is the  $i\alpha$ -th spin-orbital basis function.

For any vector  $\mathbf{u}$ ,

$$\begin{aligned} \mathbf{u}^T \mathbf{V} \mathbf{u} &= \sum_{(i\alpha,k\alpha),(l\beta,j\beta)} u_{(k\alpha,i\alpha)} V_{(i\alpha,k\alpha),(l\beta,j\beta)} u_{(l\beta,j\beta)} \\ &= \int d\vec{r}_1 d\vec{r}_2 \frac{1}{|\vec{r}_1 - \vec{r}_2|} \left( \sum_{(i\alpha,k\alpha)} u_{(k\alpha,i\alpha)} \phi_{i\alpha}^*(\vec{r}_1) \phi_{k\alpha}(\vec{r}_1) \right) \left( \sum_{(l\beta,j\beta)} u_{(l\beta,j\beta)} \phi_{j\beta}^*(\vec{r}_2) \phi_{l\beta}(\vec{r}_2) \right) \\ &= \int d\vec{r}_1 d\vec{r}_2 \frac{1}{|\vec{r}_1 - \vec{r}_2|} f(\vec{r}_1) f(\vec{r}_2) \end{aligned} \quad (33)$$

where we have substituted (32) in the second line, and define  $f(\vec{r}) \equiv \sum_{(i\alpha, k\alpha)} u_{(k\alpha, i\alpha)} \phi_{i\alpha}^*(\vec{r}) \phi_{k\alpha}(\vec{r})$ .

The Coulomb interaction  $1/|\vec{r}_1 - \vec{r}_2|$  can be further written as an integral over a Gaussian kernel, which gives

$$\frac{1}{|\vec{r}_1 - \vec{r}_2|} = \int_0^\infty dt \frac{1}{\sqrt{2\pi t^3}} e^{-\frac{|\vec{r}_1 - \vec{r}_2|^2}{2t}}. \quad (34)$$

Substituting (34) into (33), and applying the Fubini-Tonelli Theorem to exchange the integration order, we obtain

$$\mathbf{u}^T \mathbf{V} \mathbf{u} = \int_0^\infty dt \frac{1}{\sqrt{2\pi t^3}} \left( \int d\vec{r}_1 d\vec{r}_2 e^{-\frac{|\vec{r}_1 - \vec{r}_2|^2}{2t}} f(\vec{r}_1) f(\vec{r}_2) \right). \quad (35)$$

Note that the function  $f(\vec{r})$  defined here is physically well conditioned and is square-integrable, namely  $f \in L^2$ . From the basic properties of Gaussian kernels, we know that the integral in the parentheses in (35) is non-negative,

$$\int d\vec{r}_1 d\vec{r}_2 e^{-\frac{|\vec{r}_1 - \vec{r}_2|^2}{2t}} f(\vec{r}_1) f(\vec{r}_2) \geq 0, \quad (36)$$

as long as  $t > 0$ . Substituting (36) into (35), we immediately have

$$\mathbf{u}^T \mathbf{V} \mathbf{u} \geq 0, \quad (37)$$

for any  $\mathbf{u}$ . This definitively demonstrates that the *ab initio* supermatrix  $\mathbf{V}$  is positive semi-definite.

Note that for model systems such as Hubbard model, the Coulomb interaction is usually truncated or screened to a short range (or on-site) effective interaction, so that the transform from the Coulomb interaction to the Gaussian integral cannot readily be performed and thus that the above proof is not directly applicable. We indeed observe the ramifications of this fact in numerical simulations: the supermatrix of the Hubbard model is not positive semi-definite, and both negative and positive eigenvalues can appear.

## F. Tabulated Data for Figures in the Main Text

In the following, all of the data used to generate the figures in the main text are provided. It should be noted that all of the following calculations were performed by first finding a chemical potential that corresponds to a given number of electrons and then computing ED, AFQMC, and MFT energies. Depending upon the chemical potentials used, this may introduce slight deviations in the energies provided as compared with theoretically exact energies obtained within the canonical ensemble.

TABLE I. The internal energy (Hartree) of H<sub>2</sub>O in the STO-3G basis.

| $1/k_B T$ | ED         | AFQMC     | MFT        |
|-----------|------------|-----------|------------|
| 0.01      | -61.657841 | -61.66(4) | -61.564377 |
| 0.1       | -69.709056 | -69.69(4) | -69.162930 |
| 0.2       | -71.907839 | -71.90(1) | -71.516931 |
| 0.5       | -72.662457 | -72.66(1) | -72.244073 |
| 1         | -73.151258 | -73.11(2) | -72.566542 |
| 2         | -73.775883 | -73.76(2) | -73.105678 |
| 5         | -74.544744 | -74.55(2) | -74.023591 |
| 10        | -74.947094 | -74.92(2) | -74.568453 |
| 16        | -75.019015 | -74.98(3) | -74.789765 |
| 20        | -75.023360 | -75.02(3) | -74.856005 |
| 25        | -75.024138 | -75.02(4) | -74.900785 |
| 33.3      | -75.024235 | -75.02(5) | -74.932375 |

TABLE II. The internal energy (Hartree) of  $C_2$  in the STO-6G basis. The exact non-relativistic, ground state energy is -75.434537 Hartree.

| $1/k_B T$ | AFQMC       | MFT        |
|-----------|-------------|------------|
| 0.01      | -72.0633(8) | -72.043783 |
| 0.1       | -72.271(6)  | -72.103403 |
| 1         | -73.46(3)   | -72.700859 |
| 2         | -74.11(4)   | -73.274621 |
| 5         | -74.91(7)   | -74.170179 |
| 10        | -75.22(3)   | -74.646035 |
| 16        | -75.36(5)   | -74.839024 |
| 20        | -75.32(6)   | -74.882408 |
| 25        | -75.4(1)    | -74.907618 |
| 33.3      | -75.6(2)    | -74.929173 |

TABLE III: Occupancy,  $N$ , of the nitrogen atom vs. chemical potential,  $\mu$ , in the STO-6G basis at different temperatures. All temperatures and chemical potentials are in Hartree.

| $\mu$ | $N$ at $k_B T = 1.0$ | Error Bar | $N$ at $k_B T = 0.1$ | Error Bar |
|-------|----------------------|-----------|----------------------|-----------|
| -5.0  | +2.775517            | +0.015649 | +2.00000             | +0.000000 |
| -4.9  | +2.827576            | +0.017226 | +2.000001            | +0.000000 |
| -4.8  | +2.883171            | +0.009734 | +2.000004            | +0.000001 |
| -4.7  | +2.934897            | +0.016942 | +2.000007            | +0.000004 |
| -4.6  | +2.994263            | +0.016652 | +2.000016            | +0.000009 |
| -4.5  | +3.056489            | +0.018124 | +2.000024            | +0.000021 |
| -4.4  | +3.120466            | +0.016452 | +2.000123            | +0.000061 |
| -4.3  | +3.181369            | +0.021359 | +2.000364            | +0.000143 |
| -4.2  | +3.249204            | +0.018402 | +2.001005            | +0.000281 |
| -4.1  | +3.310359            | +0.023132 | +2.002860            | +0.000471 |
| -4.0  | +3.383610            | +0.011025 | +2.006538            | +0.000821 |
| -3.9  | +3.447899            | +0.022447 | +2.017944            | +0.001406 |
| -3.8  | +3.515682            | +0.018598 | +2.045490            | +0.002697 |
| -3.7  | +3.587622            | +0.012760 | +2.116417            | +0.005189 |
| -3.6  | +3.670765            | +0.019860 | +2.293460            | +0.012844 |
| -3.5  | +3.742075            | +0.024122 | +2.508752            | +0.020233 |
| -3.4  | +3.822000            | +0.018956 | +2.747936            | +0.036301 |
| -3.3  | +3.893970            | +0.017796 | +2.871995            | +0.035952 |
| -3.2  | +3.981393            | +0.024583 | +2.962444            | +0.035956 |
| -3.1  | +4.050298            | +0.017449 | +3.035517            | +0.029312 |
| -3.0  | +4.133964            | +0.026042 | +3.082995            | +0.030354 |
| -2.9  | +4.212235            | +0.025142 | +3.189069            | +0.036420 |
| -2.8  | +4.294585            | +0.029541 | +3.392010            | +0.043118 |
| -2.7  | +4.375589            | +0.017649 | +3.655683            | +0.043982 |
| -2.6  | +4.456201            | +0.026611 | +3.879189            | +0.033892 |
| -2.5  | +4.545911            | +0.022001 | +3.927999            | +0.023130 |
| -2.4  | +4.623642            | +0.021501 | +3.970532            | +0.018830 |
| -2.3  | +4.713916            | +0.029229 | +4.009007            | +0.016552 |
| -2.2  | +4.798170            | +0.028920 | +4.037212            | +0.015280 |
| -2.1  | +4.880419            | +0.029298 | +4.115878            | +0.018671 |
| -2.0  | +4.968512            | +0.024441 | +4.267119            | +0.022468 |
| -1.9  | +5.052326            | +0.022334 | +4.544293            | +0.031251 |
| -1.8  | +5.139253            | +0.030539 | +4.762987            | +0.033040 |
| -1.7  | +5.227688            | +0.051572 | +4.866220            | +0.028355 |
| -1.6  | +5.314192            | +0.018927 | +4.955101            | +0.028558 |
| -1.5  | +5.403660            | +0.021306 | +5.030537            | +0.030934 |
| -1.4  | +5.489782            | +0.025974 | +5.098210            | +0.035223 |
| -1.3  | +5.578366            | +0.028326 | +5.190183            | +0.047100 |
| -1.2  | +5.666919            | +0.032740 | +5.420303            | +0.053071 |
| -1.1  | +5.754146            | +0.020159 | +5.665965            | +0.048751 |
| -1.0  | +5.843856            | +0.011771 | +5.882139            | +0.046855 |
| -0.9  | +5.931309            | +0.026743 | +5.934199            | +0.044811 |
| -0.8  | +6.019431            | +0.034100 | +6.034486            | +0.043969 |
| -0.7  | +6.107615            | +0.028906 | +6.106881            | +0.062831 |
| -0.6  | +6.195266            | +0.017643 | +6.149598            | +0.072681 |

|      |           |           |           |           |
|------|-----------|-----------|-----------|-----------|
| -0.5 | +6.281296 | +0.028198 | +6.406233 | +0.093832 |
| -0.4 | +6.372849 | +0.029871 | +6.583948 | +0.103595 |
| -0.3 | +6.459179 | +0.038297 | +6.786758 | +0.068000 |
| -0.2 | +6.547036 | +0.032811 | +6.918219 | +0.077881 |
| -0.1 | +6.633839 | +0.018306 | +6.965226 | +0.034042 |
| +0.0 | +6.722513 | +0.026833 | +7.008555 | +0.034042 |
| +0.1 | +6.806090 | +0.029384 | +7.116937 | +0.056651 |
| +0.2 | +6.898661 | +0.027031 | +7.368022 | +0.145205 |
| +0.3 | +6.982928 | +0.034052 | +7.461403 | +0.143748 |
| +0.4 | +7.063049 | +0.040539 | +7.843200 | +0.124731 |
| +0.5 | +7.153682 | +0.027810 | +7.985141 | +0.107265 |
| +0.6 | +7.238487 | +0.037560 | +8.038756 | +0.078324 |
| +0.7 | +7.327173 | +0.029914 | +8.016139 | +0.028747 |
| +0.8 | +7.412065 | +0.022930 | +8.063458 | +0.025271 |
| +0.9 | +7.489670 | +0.021011 | +8.120954 | +0.096210 |
| +1.0 | +7.570864 | +0.020641 | +8.255501 | +0.192727 |
| +1.1 | +7.658912 | +0.011750 | +8.709194 | +0.135730 |
| +1.2 | +7.736232 | +0.027300 | +8.817749 | +0.091703 |
| +1.3 | +7.822420 | +0.018079 | +8.994548 | +0.048407 |
| +1.4 | +7.898839 | +0.014423 | +9.026712 | +0.046844 |
| +1.5 | +7.974030 | +0.034715 | +9.041305 | +0.041363 |
| +1.6 | +8.056038 | +0.014513 | +9.090873 | +0.039118 |
| +1.7 | +8.135464 | +0.032067 | +9.208324 | +0.035563 |
| +1.8 | +8.208452 | +0.021635 | +9.482027 | +0.021857 |
| +1.9 | +8.286496 | +0.017512 | +9.674730 | +0.012889 |
| +2.0 | +8.356670 | +0.010235 | +9.860978 | +0.005590 |
| +2.1 | +8.426331 | +0.031939 | +9.946095 | +0.002697 |
| +2.2 | +8.501034 | +0.015649 | +9.977586 | +0.001392 |
| +2.3 | +8.574974 | +0.016645 | +9.991786 | +0.001019 |
| +2.4 | +8.640520 | +0.015122 | +9.997221 | +0.000455 |
| +2.5 | +8.706805 | +0.016108 | +9.998957 | +0.000274 |
| +2.6 | +8.771075 | +0.015997 | +9.999569 | +0.000133 |
| +2.7 | +8.840801 | +0.023600 | +9.999879 | +0.000060 |
| +2.8 | +8.900054 | +0.015195 | +9.999953 | +0.000022 |
| +2.9 | +8.963548 | +0.021800 | +9.999999 | +0.000008 |
| +3.0 | +9.018084 | +0.011670 | +9.999992 | +0.000003 |
| +3.1 | +9.081703 | +0.012430 | +9.999999 | +0.000001 |
| +3.2 | +9.135721 | +0.015993 | +9.999999 | +0.000001 |
| +3.3 | +9.187430 | +0.016366 | +9.999999 | +0.000000 |
| +3.4 | +9.240778 | +0.013390 | +10.00000 | +0.00000  |
| +3.5 | +9.287409 | +0.011733 | +10.00000 | +0.00000  |
| +3.6 | +9.337543 | +0.016078 | +10.00000 | +0.00000  |
| +3.7 | +9.380295 | +0.008802 | +10.00000 | +0.00000  |
| +3.8 | +9.422328 | +0.007795 | +10.00000 | +0.00000  |
| +3.9 | +9.462889 | +0.009757 | +10.00000 | +0.00000  |
| +4.0 | +9.499485 | +0.010482 | +10.00000 | +0.00000  |

TABLE IV. The internal energy (Hartree) of  $H_{10}$  in the STO-6G basis at its equilibrium bond length of 1.786 a.u. The exact, non-relativistic ground state energy is -5.424570 Hartree.

| $1/k_B T$ | AFQMC     | MFT       |
|-----------|-----------|-----------|
| 0.01      | 0.0803(9) | 0.093683  |
| 0.1       | -0.151(4) | -0.027001 |
| 1         | -2.01(1)  | -1.219754 |
| 2         | -3.29(2)  | -2.353559 |
| 5         | -4.77(3)  | -4.105092 |
| 10        | -5.30(5)  | -4.841360 |
| 16        | -5.38(4)  | -5.059083 |
| 20        | -5.38(2)  | -5.117851 |
| 25        | -5.44(6)  | -5.161809 |
| 33.3      | -5.41(2)  | -5.204183 |

TABLE V. The internal energy (Hartree) of  $H_{10}$  in the STO-6G basis at a stretched bond length of 2.4 a.u. The exact non-relativistic, ground state energy is -5.227936 Hartree.

| $1/k_B T$ | AFQMC      | MFT       |
|-----------|------------|-----------|
| 0.01      | -1.7488(2) | -1.739656 |
| 0.1       | -1.865(1)  | -1.773753 |
| 0.2       | -1.981(3)  | -1.811868 |
| 0.5       | -2.287(4)  | -1.927442 |
| 1         | -2.723(9)  | -2.122643 |
| 2         | -3.41(3)   | -2.510962 |
| 5         | -4.38(3)   | -3.483536 |
| 10        | -4.91(4)   | -4.289207 |
| 16        | -5.14(4)   | -4.620001 |
| 20        | -5.13(3)   | -4.714858 |
| 25        | -5.19(5)   | -4.780650 |
| 33.3      | -5.2(1)    | -4.837063 |

TABLE VI. The internal energy of a  $4 \times 2$  single-band Hubbard model with  $U/t = 4$  at half filling on a square lattice. All energies are in units of  $t$ .

| $1/k_B T$ | AFQMC   | MFT       |
|-----------|---------|-----------|
| 0.01      | 7.80(2) | 7.880007  |
| 0.1       | 6.03(3) | 6.806939  |
| 1         | -2.8(2) | -0.203592 |
| 2         | -4.3(1) | -2.539894 |
| 4         | -5.7(1) | -3.784092 |
| 10        | -5.9(1) | -3.999455 |
| 20        | -5.9(1) | -4.000000 |
| 25        | -6.0(1) | -4.000000 |

TABLE VII. The internal energy of a  $4 \times 2$  two-band Hubbard-Kanamori model with  $U/t = 4, J/t = 1$  at half filling on a square lattice. All energies are in units of  $t$ .

| $1/k_B T$ | AFQMC    | MFT       |
|-----------|----------|-----------|
| 0.01      | 27.53(6) | 27.760014 |
| 0.1       | 23.5(1)  | 25.613879 |
| 1         | 5.2(3)   | 11.592815 |
| 2         | 1.1(5)   | 6.920213  |
| 4         | -1.1(3)  | 4.431817  |
| 10        | -0.8 (6) | 4.001090  |
| 16        | -0.6 (5) | 4.000003  |

TABLE VIII. Average absolute value of the phase angle (Degrees) for various *ab initio* systems at different temperatures, under free propagation and background subtraction. Slashes indicate that error bars were not able to be converged for the given system.

| $1/k_B T$ | Free Propagation |                | Background Subtraction |                |                               |                             |
|-----------|------------------|----------------|------------------------|----------------|-------------------------------|-----------------------------|
|           | H <sub>2</sub> O | C <sub>2</sub> | H <sub>2</sub> O       | C <sub>2</sub> | H <sub>10</sub> (Equilibrium) | H <sub>10</sub> (Stretched) |
| 0.01      | 41.8(9)          | 26.3(6)        | 0.030(2)               | 4.3(5)E-6      | 5.3(1)E-4                     | 3.9(1)E-6                   |
| 1         | 91(2)            | 89(2)          | 3.4(7)                 | 0.6(3)         | 1.03(4)                       | 0.40(1)                     |
| 2         | 89(2)            | 89(2)          | 8(1)                   | 2.2(8)         | 3.6(1)                        | 1.58(5)                     |
| 5         | /                | /              | 27(1)                  | 11(1)          | 14.4(6)                       | 10.9(3)                     |
| 10        | /                | /              | 46(1)                  | 29(2)          | 28.4(7)                       | 29.5(6)                     |
| 16        | /                | /              | 53(1)                  | 56(2)          | 37.7(7)                       | 41.6(7)                     |
| 20        | /                | /              | 57(1)                  | 74(2)          | 40.2(7)                       | 57.1(9)                     |
| 25        | /                | /              | 58(1)                  | 73(2)          | 54.2(8)                       | 50.6(8)                     |
| 33.3      | /                | /              | 64(1)                  | 75(1)          | 53.2(9)                       | 74(1)                       |

### G. Tabulated Data for Other First and Second Row Atoms and Molecules

Benchmark results for other first and second row atoms in the periodic table not discussed in the text and  $\text{H}_2$  are provided below at various inverse temperatures, computed using ED, AFQMC, and MFT.

TABLE IX. The internal energy (Hartree) of  $\text{H}_2$  in the STO-3G Basis.

| $1/k_B T$ | ED        | AFQMC      | MFT       |
|-----------|-----------|------------|-----------|
| 0.01      | -0.608951 | -0.6090(1) | -0.608298 |
| 0.1       | -0.616675 | -0.6168(4) | -0.610226 |
| 1         | -0.686456 | -0.6862(6) | -0.629880 |
| 5         | -0.870669 | -0.871(2)  | -0.720445 |
| 10        | -0.974220 | -0.972(3)  | -0.823580 |
| 20        | -1.048646 | -1.047(4)  | -0.957009 |
| 50        | -1.066490 | -1.069(2)  | -1.038881 |
| 100       | -1.066602 | -1.072(7)  | -1.041605 |

TABLE X. The internal energy (Hartree) of the helium atom in the MIDI Basis.

| $1/k_B T$ | ED        | AFQMC      | MFT       |
|-----------|-----------|------------|-----------|
| 0.01      | -0.212171 | -0.2118(7) | -0.207955 |
| 0.1       | -0.370275 | -0.366(3)  | -0.327364 |
| 0.2       | -0.545960 | -0.543(2)  | -0.460965 |
| 0.5       | -1.047245 | -1.036(6)  | -0.858395 |
| 1         | -1.722136 | -1.715(5)  | -1.462187 |
| 2         | -2.502106 | -2.506(5)  | -2.276931 |
| 5         | -2.846430 | -2.846(3)  | -2.813331 |
| 10        | -2.850574 | -2.851(4)  | -2.835515 |
| 20        | -2.850577 | -2.851(5)  | -2.835598 |
| 50        | -2.850577 | -2.853(5)  | -2.835598 |

TABLE XI. The internal energy (Hartree) of the lithium atom in the MIDI Basis.

| $\beta$ | ED        | AFQMC      | MFT       |
|---------|-----------|------------|-----------|
| 0.01    | -4.527322 | -4.527(2)  | -4.524944 |
| 0.05    | -4.650689 | -4.650(3)  | -4.637345 |
| 0.1     | -4.800995 | -4.801(5)  | -4.771334 |
| 0.2     | -5.085673 | -5.084(8)  | -5.018451 |
| 0.5     | -5.787149 | -5.79(1)   | -5.615290 |
| 1       | -6.535186 | -6.528(7)  | -6.270235 |
| 2       | -7.152696 | -7.148(5)  | -6.920131 |
| 5       | -7.288515 | -7.2808(6) | -7.253609 |
| 10      | -7.335787 | -7.3218(6) | -7.289847 |
| 20      | -7.387277 | -7.367(1)  | -7.328862 |
| 50      | -7.415739 | -7.385(3)  | -7.365749 |
| 100     | -7.418664 | -7.384(2)  | -7.393584 |

TABLE XII. The internal energy (Hartree) of the boron atom in the MIDI Basis.

| $\beta$ | ED         | AFQMC      | MFT        |
|---------|------------|------------|------------|
| 0.01    | -11.082440 | -11.08(1)  | -11.080260 |
| 0.1     | -13.917083 | -13.93(4)  | -13.752883 |
| 0.2     | -16.875802 | -16.88(5)  | -16.377219 |
| 0.5     | -21.866141 | -21.85(3)  | -21.033821 |
| 1       | -23.240278 | -23.236(9) | -22.891464 |
| 2       | -23.591185 | -23.57(1)  | -23.236813 |
| 5       | -24.100273 | -24.08(2)  | -23.722880 |
| 10      | -24.336156 | -24.32(3)  | -24.021959 |
| 20      | -24.426170 | -24.4(1)   | -24.198037 |
| 50      | -24.455867 | -24.6(3)   | -24.250785 |
| 100     | -24.462663 | -24.3(2)   | -24.273218 |

TABLE XIII. The internal energy (Hartree) of the carbon atom in the MIDI Basis. The slash indicates that numerical underflow or overflow occurs at the corresponding temperature.

| $\beta$ | ED         | AFQMC     | MFT        |
|---------|------------|-----------|------------|
| 0.01    | -19.206839 | -19.22(2) | -19.191994 |
| 0.1     | -25.185109 | -25.17(6) | -24.725267 |
| 0.2     | -30.220594 | -30.19(6) | -29.280635 |
| 0.5     | -35.001762 | -34.91(1) | -34.271457 |
| 1       | -35.742693 | -35.75(1) | -35.225802 |
| 2       | -36.444645 | -36.43(2) | -35.843619 |
| 5       | -37.231883 | -37.23(3) | -36.731085 |
| 10      | -37.435310 | -37.50(6) | -37.011903 |
| 20      | -37.498072 | -37.6(4)  | -37.078776 |
| 50      | -37.512651 | -37.4(3)  | -37.081044 |
| 100     | -37.514843 | /         | -37.081044 |

TABLE XIV. The internal energy (Hartree) of the nitrogen atom in the MIDI Basis. The slash indicates that numerical underflow or overflow occurs at the corresponding temperature.

| $\beta$ | ED         | AFQMC     | MFT        |
|---------|------------|-----------|------------|
| 0.01    | -30.592444 | -30.60(2) | -30.552265 |
| 0.1     | -41.066521 | -41.05(7) | -40.218672 |
| 0.2     | -47.408502 | -47.39(4) | -46.282256 |
| 0.5     | -50.717899 | -50.70(2) | -50.074317 |
| 1       | -51.729096 | -51.69(2) | -50.946742 |
| 2       | -52.956080 | -52.94(2) | -52.183746 |
| 5       | -53.891886 | -54.00(3) | -53.340733 |
| 10      | -54.047597 | -54.0(1)  | -53.499021 |
| 20      | -54.109484 | -53.6(6)  | -53.515755 |
| 33.3    | -54.136716 | -54.2(4)  | -53.519663 |
| 50      | -54.153396 | -53.9(5)  | -53.526544 |
| 100     | -54.167023 | /         | -53.559940 |

TABLE XV. The internal energy (Hartree) of the oxygen atom in the MIDI Basis. The slash indicates that numerical underflow or overflow occurs at the corresponding temperature.

| $\beta$ | ED         | AFQMC     | MFT        |
|---------|------------|-----------|------------|
| 0.01    | -46.029567 | -46.03(6) | -45.948682 |
| 0.1     | -61.673823 | -61.67(7) | -60.517364 |
| 0.2     | -67.666379 | -67.66(3) | -66.682083 |
| 0.5     | -69.976063 | -69.95(2) | -69.122111 |
| 1       | -71.532594 | -71.50(3) | -70.513328 |
| 2       | -73.308290 | -73.32(3) | -72.441522 |
| 5       | -74.307581 | -74.35(4) | -73.756461 |
| 10      | -74.406445 | -74.3(1)  | -73.824955 |
| 20      | -74.435497 | -74.4(3)  | -73.827113 |
| 33.3    | -74.441517 | -73.7(6)  | -73.827118 |
| 50      | -74.443573 | /         | -73.827118 |
| 100     | -74.444625 | /         | /          |

TABLE XVI. The internal energy (Hartree) of the fluorine atom in the MIDI Basis. The slash indicates that numerical underflow or overflow occurs at the corresponding temperature.

| $\beta$ | ED         | AFQMC     | MFT        |
|---------|------------|-----------|------------|
| 0.01    | -65.761204 | -65.76(5) | -65.618951 |
| 0.1     | -86.145314 | -86.12(7) | -84.901888 |
| 0.2     | -90.802146 | -90.78(2) | -89.992038 |
| 0.5     | -93.122699 | -93.09(3) | -92.028526 |
| 1       | -95.473340 | -95.44(4) | -94.288254 |
| 2       | -97.893048 | -97.90(3) | -97.038210 |
| 5       | -98.862027 | -98.83(3) | -98.446321 |
| 10      | -98.922403 | -98.9(1)  | -98.473558 |
| 20      | -98.936059 | -98.8(2)  | -98.474385 |
| 25      | -98.936614 | -99.1(4)  | -98.474813 |
| 33.3    | -98.936928 | /         | -98.475728 |
| 50      | -98.937363 | /         | -98.478298 |
| 100     | -98.938512 | /         | -98.490596 |

TABLE XVII. The internal energy (Hartree) of the neon atom in the MIDI Basis. The slash indicates that numerical underflow or overflow occurs at the corresponding temperature.

| $\beta$ | ED          | AFQMC       | MFT         |
|---------|-------------|-------------|-------------|
| 0.01    | -115.219180 | -115.218(3) | -115.154574 |
| 0.1     | -116.435430 | -116.43(1)  | -115.913272 |
| 0.2     | -117.606155 | -117.60(2)  | -116.752691 |
| 0.5     | -120.446996 | -120.43(3)  | -119.149895 |
| 1       | -123.662816 | -123.62(4)  | -122.371375 |
| 2       | -126.701453 | -126.69(3)  | -125.813576 |
| 5       | -127.889630 | -127.88(2)  | -127.649640 |
| 10      | -127.905179 | -127.88(4)  | -127.757574 |
| 20      | -127.905199 | -127.92(5)  | -127.758803 |
| 50      | -127.905199 | -127.9(1)   | -127.758803 |
| 100     | -127.905199 | /           | -127.758803 |

## H. Computational Scaling

As mentioned in the main text, our method scales as  $O(N^3)$ – $O(N^4)$ , where  $N$  is the number of orbitals (basis set size). As with most quantum Monte Carlo algorithms, this scaling stems from the fact that our algorithm requires a large number of matrix multiplications, inversions (using LU factorization), and diagonalizations, all of which have an  $O(N^3)$  scaling. The CPU time vs. the number of orbitals for several systems is summarized and plotted with a log scale in Figure 1 below, illustrating a typical quantum Monte Carlo power law scaling.

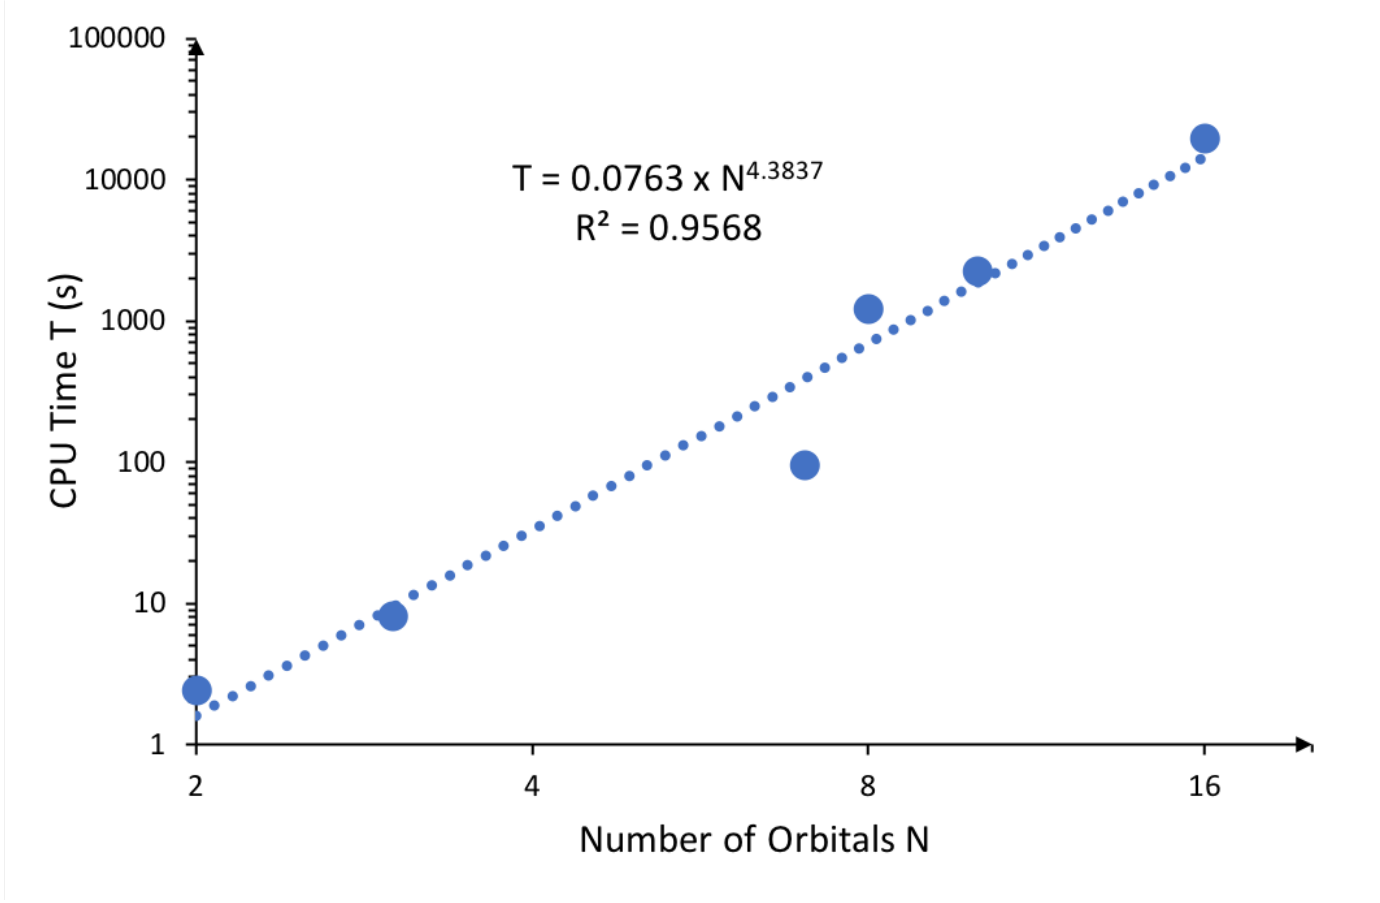

FIG. 1. CPU time vs. number of orbitals for H<sub>2</sub> (STO-3G, N=2), Be (MIDI, N=3), H<sub>2</sub>O (STO-3G, N=7), C<sub>2</sub>(STO-6G, N=8), H<sub>10</sub> (STO-6G, N=10), and the 4x2 2-orbital Hubbard-Kanamori model (N=16) at  $\beta = 1$ ,  $\Delta\tau = 0.05$  with 128 walkers and 10 blocks, where  $N$  is the total number of orbitals in the basis. Dashed line is a fitting that illustrates power law scaling. Note that the y-axis is given using a log scale.

### I. Calculation of Statistical Errors

In our finite temperature AFQMC, each walker samples the auxiliary field space and carries information about physical observables. We call propagation in imaginary time from inverse temperature 0 to  $\beta$  one *block*. The calculation is repeated  $M$  times to get  $M$  blocks, and  $N$  *walkers* are used per block. To calculate the error bar on physical observables (internal energy in our case), we first average the internal energy over all  $N$  walkers within each block as  $E_i$ , where  $i = 1, 2, \dots, M$ . Then, from standard error analysis, the error bar on the average internal energy is obtained as

$$\sigma = \sqrt{\frac{\sum_{i=1}^M (E_i - \bar{E})^2}{(M-1)M}}, \quad (38)$$

where  $\bar{E}$  is the mean of the internal energy. Note that, while more sophisticated error analyses that address correlations among samples, such as reblocking, exist, we believe that our simple model of statistical independence will still provide sound observable estimates.
